# Supplementary material for: Amortized variance reduction for doubly stochastic objectives
Source: arXiv:2003.04125 source file (2020-03-09)
Supplement: Supplementary file 1 [file appendix_theoretical.tex]

\section{CONVERGENCE OF THE PROPOSED METHOD}
\label{appx:appendix_a}

\begin{proof}[Proof of Theorem~\ref{T:Convergence}]
We first establish the following lemma based on the smoothness and strong convexity of $f(\vepsilon,\params)$.
\begin{lemma}
By smoothness (Assumption 1) and strong convexity (Assumption 2) of $f(\vepsilon,\params)$, we have
\begin{eqnarray}
\E [f(\vepsilon,\params)- f(\vepsilon,\params^*)] \ge \frac{1}{2L}\E\bigg[\|\nabla f(\vepsilon,\params) -\nabla f(\vepsilon,\params^*)\|_2^2\bigg].
\end{eqnarray}
\end{lemma}

Let
$h(\vepsilon,\params) = f(\vepsilon,\params) - f(\vepsilon,\params^*) - \nabla f(\vepsilon,\params^*)^\T(\params-\params^*)$. By convexity of $f(\vepsilon,\params)$ we know that $h(\vepsilon,\params) \ge 0$. Let $\params'=\params-\eta\nabla h(\vepsilon,\params))$.
Notice that $\nabla h(\vepsilon,\params)=  \nabla f(\vepsilon,\params) -\nabla f(\vepsilon,\params^*)$.

\begin{eqnarray}\nn
h(\vepsilon,\params')- h(\vepsilon,\params) &\le& -\eta\nabla h(\vepsilon,\params)\transpose \nabla h(\vepsilon,\params) + \frac{1}{2}L\eta^2\|\nabla h(\vepsilon,\params))\|_2^2\\\nn
&=&\big(\frac{1}{2}L\eta^2-\eta\big)\|\nabla h(w,\epsilon))\|_2^2.
\end{eqnarray}

With the choice of $\eta=\frac{1}{L}$
and noticing $h(\vepsilon,\params') \ge 0$:
\begin{eqnarray}\nn
- h(\vepsilon,\params) \le -\frac{1}{2L}\|\nabla h(\vepsilon,\params))\|_2^2.
\end{eqnarray}
Taking expectations, we have
\begin{eqnarray}\nn
\frac{1}{2L}\E[\|\nabla h(\vepsilon,\params))\|_2^2] &\le& \E[ h(\vepsilon,\params)]\\\nn
&=& \E[f(\vepsilon,\params) - f(\vepsilon,\params^*) - \nabla f(\vepsilon,\params^*)^\T(\params-\params^*)]\\\nn
&\le& \E[f(\vepsilon,\params) - f(\vepsilon,\params^*)] ,
\end{eqnarray}
which completes the proof of this lemma. \\

Now, let $v_t=\nabla f(\vepsilon_{t-1},\params_{t-1})-c(\vepsilon_{t-1},\params_{t-1})$. Then
\begin{eqnarray}\nn
&&\hspace{-3em}\E [\|\params_t-\params^*\|_2^2] \\\nn
&=& \|\params_{t-1}-\params^*\|_2^2 - 2\eta (\params_{t-1}-\params^*)^\T\E [v_t] + \eta^2\E [\|v_t\|_2^2]\\\nn
&=&  \|\params_{t-1}-\params^*\|_2^2 - 2\eta (\params_{t-1}-\params^*)^\T\E[\nabla f(\vepsilon_{t-1},\params_{t-1})] + \eta^2\E [\|v_t\|_2^2] \\\label{in1}
&\le& \|\params_{t-1}-\params^*\|_2^2 -2\eta \E[ [f(\vepsilon,\params_{t-1}) -  f(\vepsilon,\params^*) ] + \eta^2\E[ \|v_t\|_2^2] .
\end{eqnarray}

For the last term $\E [\|v_t\|_2^2]$, we have
\begin{eqnarray}\nn
&&\hspace{-3em}\E [\|v_t\|_2^2]\\\nn
&=& \E\bigg[ \| \nabla f(\vepsilon_{t-1},\params_{t-1}) - \nabla f(\vepsilon_{t-1},\params^*) +\nabla f(\vepsilon_{t-1},\params^*) - c(\vepsilon_{t-1},\params_{t-1})\|^2   \bigg]\\\nn
&\le&2\E\bigg[\|\nabla f(\vepsilon_{t-1},\params_{t-1}) - \nabla f(\vepsilon_{t-1},\params^*)\|_2^2\bigg] \\\nn
&&~~~+ 2\E\bigg[\|\nabla f(\vepsilon_{t-1},\params^*) - c(\vepsilon_{t-1},\params_{t-1})\|_2^2\bigg]\\\label{in2}
&\le& (4L+2M) \E [f(\vepsilon_{t-1},\params_{t-1})- f(\vepsilon_{t-1},\params^*)] ,
\end{eqnarray}
where the last inequality holds by Assumption 3. 

By strong convexity of $f(\vepsilon, \params)$, we have
\begin{eqnarray}\label{in3}
\|\params_{t-1} - \params^*\|_2^2 \le \frac{2}{H} f(\vepsilon,\params_{t-1}) - f(\vepsilon,\params^*).
\end{eqnarray}

Combining the last 3 inequalities we get
\begin{eqnarray}\nn
&&\hspace{-2em}\E[\|\params_t-\params^*\|_2^2] \\\nn
&\le&\E [\|\params_{t-1}-\params^*\|_2^2] - 2\eta(1-\eta(2L+M))\E [f(\vepsilon,\params_{t-1}) -  f(\vepsilon,\params^*) ] \\\nn
&\le& \Big(1-\eta H(1-\eta(2L+M))\Big)\E [\|\params_{t-1}-\params^*\|_2^2] .
\end{eqnarray}

For
$\eta \le \frac{1}{2L+M}$ and 
$c = (1-\eta H(1-\eta(2L+M)) $, we have
\begin{eqnarray}\nn
\E[\|\params_t-\params^*\|_2^2] \le c^t \|\params_0-\params^*\|_2^2,
\end{eqnarray}
which completes the proof of Theorem~\ref{T:Convergence}.

% For
% $\eta = \frac{1}{2(2L+M)}$ and 
% $c = 1-\frac{H}{4(2L+M)}$, we have
% \begin{eqnarray}
% \E[\|\theta_t-\theta^*\|_2^2] \le c^t \|\theta_0-\theta^*\|_2^2
% \end{eqnarray}

When Assumption 3 does not hold and Assumption 4 holds, following the same line of reasoning and replacing the upper bound on $\E\bigg[\|\nabla f(\vepsilon_{t-1},\params^*) - c(\vepsilon_{t-1},\params_{t-1})\|_2^2\bigg]$ with $\bar{M}$, we have
\begin{eqnarray}\nn
&&\hspace{-3em}\E [\|v_t\|_2^2]\\\nn
&=& \E\bigg[ \| \nabla f(\vepsilon_{t-1},\params_{t-1}) - \nabla f(\vepsilon_{t-1},\params^*) +\nabla f(\vepsilon_{t-1},\params^*) - c(\vepsilon_{t-1},\params_{t-1})\|^2   \bigg]\\\nn
&\le&2\E\bigg[\|\nabla f(\vepsilon_{t-1},\params_{t-1}) - \nabla f(\vepsilon_{t-1},\params^*)\|_2^2\bigg] \\\nn
&&~~~+ 2\E\bigg[\|\nabla f(\vepsilon_{t-1},\params^*) - c(\vepsilon_{t-1},\params_{t-1})\|_2^2\bigg]\\\label{in4}
&\le& 4L \E [f(\vepsilon_{t-1},\params_{t-1})- f(\vepsilon_{t-1},\params^*)] + 2\bar{M}.
\end{eqnarray}

Combining inequalities~\eqref{in1}, \eqref{in3} and~\eqref{in4}, we have
\begin{eqnarray}\nn
&&\hspace{-2em}\E[\|\params_t-\params^*\|_2^2] \\\nn
&\le& \bigg(1-\eta H(1-2L\eta)\bigg)\E [\|\params_{t-1}-\params^*\|_2^2] + 2\eta^2\bar{M}.
\end{eqnarray}

For
$\eta \le \frac{1}{2L}$ and 
$\bar{c} = (1-\eta H(1-2L\eta) )$, we have
\begin{eqnarray}\nn
\E[\|\params_t-\params^*\|_2^2] 
\le \bar{c} \,\E [\|\params_{t-1}-\params^*\|_2^2] + 2\eta^2\bar{M}.
\end{eqnarray}\nn
Equivalently, 
\begin{eqnarray}\nn
\E[\|\params_t-\params^*\|_2^2] + \frac{2\eta^2\bar{M}}{\bar{c}-1}
\le \bar{c}\bigg(\E [\|\params_{t-1}-\params^*\|_2^2] +\frac{2\eta^2\bar{M}}{\bar{c}-1}\bigg),
\end{eqnarray}\nn
which shows
\begin{eqnarray}\nn
\E[\|\params_t-\params^*\|_2^2] + \frac{2\eta^2\bar{M}}{\bar{c}-1}
\le \bar{c}^t\bigg(\|\params_{0}-\params^*\|_2^2 +\frac{2\eta^2\bar{M}}{\bar{c}-1}\bigg).
\end{eqnarray}\nn
Thus, for the $\E[\|\theta_t-\theta^*\|^2_2]$, we have
\begin{eqnarray}\nn
\E[\|\params_t-\params^*\|_2^2] 
\le \bar{c}^t\|\params_{0}-\params^*\|_2^2 +\frac{2\eta^2\bar{M}(\bar{c}^t-1)}{\bar{c}-1}.
\end{eqnarray}\nn

\end{proof}

\clearpage
